# Supplementary material for: Emergence of half-metallic ferromagnetism and valley polarization in transition metal substituted WSTe monolayer
Source: arXiv:2412.10819 source file (2024-12-14)
Supplement: Supplementary file 1 [file Supplemental_Material.pdf]

# Supporting Information: Emergence of half-metallic ferromagnetism and valley polarization in transition metal substituted WSTe monolayer

Shivani Kumawat,[1] Chandan Kumar Vishwakarma,[2] Mohd Zeeshan,[1] Indranil Mal,[1] Sunil Kumar,[1, *] and B. K. Mani[1, †]

[1]*Department of Physics, Indian Institute of Technology, Hauz Khas, New Delhi 110016, India*

[2]*Materials Department, University of California, Santa Barbara, California 93106-5050, USA*

## I. ELECTRONIC BAND STRUCTURE

Fig. 1 and Fig. 2 show the spin-polarized electronic band structure of Mn and Co-WSTe systems, respectively, where the upper panel shows the spin-up channel, while the lower panel indicates the spin-down channel. As clearly shown from the Fig. 1, for 6.25, 12.5 and 18.75% concentration of Mn, we observe semiconducting behaviour for both of the spin channels, while 25% concentration shows half metallic nature. The spin-down band gap for all concentrations is relatively higher than the spin-up channel, as given in the main paper.

For Co-substituted WSTe, as shown in Fig. 2, for 6.25 and 12.5% concentration of Co, we observe a semiconducting behavior for both spin-up and spin-down channels. However, for 18.75 and 25% concentration, we observe a metallic behavior in the spin-up channel, whereas the spin down channel exhibits a semiconducting nature with band gaps of 0.59 and 0.33 eV, respectively.

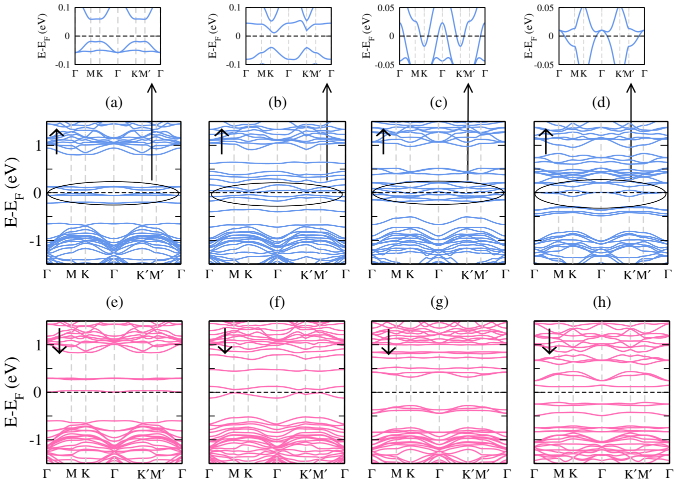


FIG. 2. Spin polarised band structure of Co-WSTe with various Mn concentrations (a) 6.25%, (b) 12.5%, (c) 18.75%, and (d) 25%. The upper panel shows the spin-up channel, and the lower panel (e,f,g,h) shows the spin-down channels. The Fermi level is set to 0 eV.

## II. VALLEY POLARIZATION

Fig. 3 shows the electronic band structure of Co-WSTe (panel (a)) and Mn-WSTe (panel (b)) in the presence of

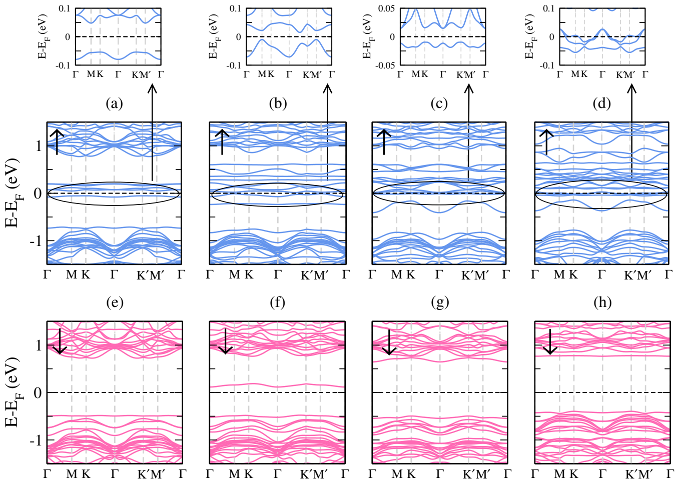


FIG. 1. Spin polarised band structure of Mn-WSTe with various Mn concentrations (a) 6.25%, (b) 12.5%, (c) 18.75%, and (d) 25%. The upper panel shows the spin-up channel, and the lower panel (e,f,g,h) shows the spin-down channels. The Fermi level is set to 0 eV.

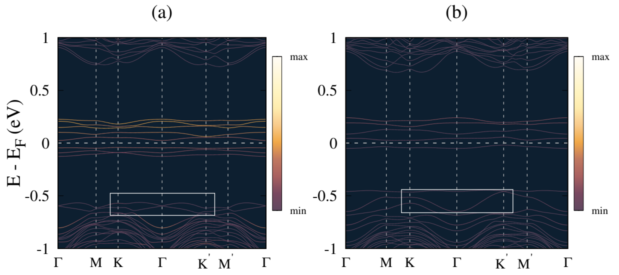


FIG. 3. Atom-projected band structures of (a) Co-doped WSTe and (b) Mn-doped WSTe, with the color bar indicating contributions from Co and Mn atoms, respectively. The highlighted box marks the selected band used for valley polarization calculations, with the Fermi level aligned at 0 eV.

SOC for 6.25% concentration. As similar to Fe-WSTe, the defect states emerge in the vicinity of the Fermi level of the bands. These defect states mainly comprise of W and TM atoms, which suggests a strong orbital hybridization between these atoms. The spin degeneracy in the bands is lifted, that gives the valley polarization of 46.3 and 54.4 meV for Co- and Mn-WSTe, respectively.

Next, we investigate the effect of uniaxial and biaxial strain on the valley polarization properties of Mn and Co-

* kumarsunil@physics.iitd.ac.in
† bkmani@physics.iitd.ac.in

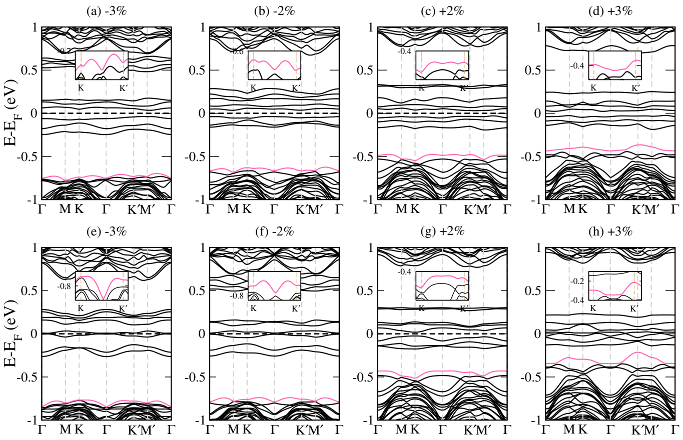


FIG. 4. Electronic structures of Co-WSTe (a)-(d) correspond to the uniaxial compressive and tensile strain of -3, -2, +2, and +3%, respectively. (e)-(h) correspond to the biaxial compressive and tensile strain of -3, -2, +2 and +3%, respectively.

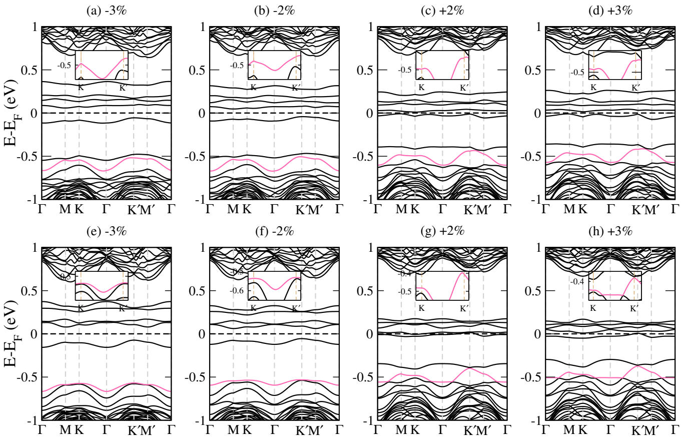


FIG. 5. Electronic structures of Mn-WSTe (a)-(d) correspond to the uniaxial compressive and tensile strain of -3, -2, +2, and +3%, respectively. (e)-(h) correspond to the biaxial compressive and tensile strain of -3, -2, +2 and +3%, respectively.

WSTe. Fig. 4 and Fig. 5 demonstrates the electronic band structure of 6.25% Co-WSTe and 6.25% Mn-WSTe under uniaxial strain (panel (a-d)), and biaxial strain (panel (e-h)).

Table I represents the valley polarization values ($\Delta_{KK'}$ (meV)). Under uniaxial strain, Co-substitution shows an increase in valley polarization from -3% to +2% strain, however it shows sudden drop for +3%. In contrast, Mn-substitution shows increasing valley polarization with tensile strain and decreasing valley polarization with compressive strain. This type of trend is consistent with Fe-WSTe. Under biaxial strain, both Co and Mn experience a rise in polarization with positive strain, especially at +3%, where Mn and Co achieves the maximum polarization of 98.1 and 81.3 meV, respectively. These results highlight the distinct strain-dependent valley polarization behavior in Co and Mn-WSTe, indicating the potential for tuning valleytronic properties through specific substitution and strain engineering.

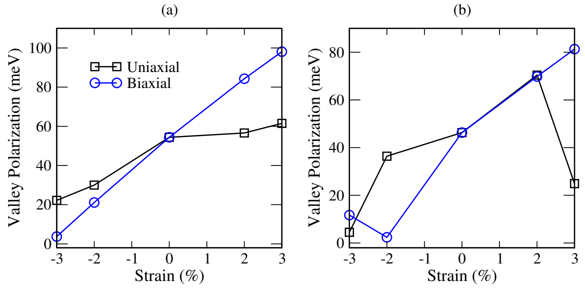


FIG. 6. Valley polarization as a function of uniaxial and biaxial strain for (a) Mn and, (b) Co-WSTe, respectively.

TABLE I. Valley polarization at different uniaxial and biaxial strains for 6.25% Fe-WSTe.

| Uniaxial strain | $\Delta_{KK'}$ (meV) | | Biaxial strain | $\Delta_{KK'}$ (meV) | |
|---|---|---|---|---|---|
| | Co | Mn | | Co | Mn |
| -3 | 4.5 | 22.2 | -3 | 11.7 | 3.7 |
| -2 | 36.1 | 30.0 | -2 | 2.4 | 21.1 |
| 0 | 46.3 | 54.4 | 0 | 46.3 | 54.4 |
| 2 | 70.4 | 56.6 | 2 | 69.8 | 84.3 |
| 3 | 24.9 | 61.5 | 3 | 81.3 | 98.1 |
